# Supplementary material for: HyperFields: Towards Zero-Shot Generation of NeRFs from Text
Source: arXiv:2310.17075 source file (2024-06-13)
Supplement: Supplementary file 1 [file supplementary.tex]

% The \author macro works with any number of authors. There are two commands
% used to separate the names and addresses of multiple authors: \And and \AND.
%
% Using \And between authors leaves it to LaTeX to determine where to break the
% lines. Using \AND forces a line break at that point. So, if LaTeX puts 3 of 4
% authors names on the first line, and the last on the second line, try using
% \AND instead of \And before the third author name.

%\title{Placeholder}
%\begin{document}

% \twocolumn[{%
% \renewcommand\twocolumn[1][]{#1}%
% \maketitle
% \input{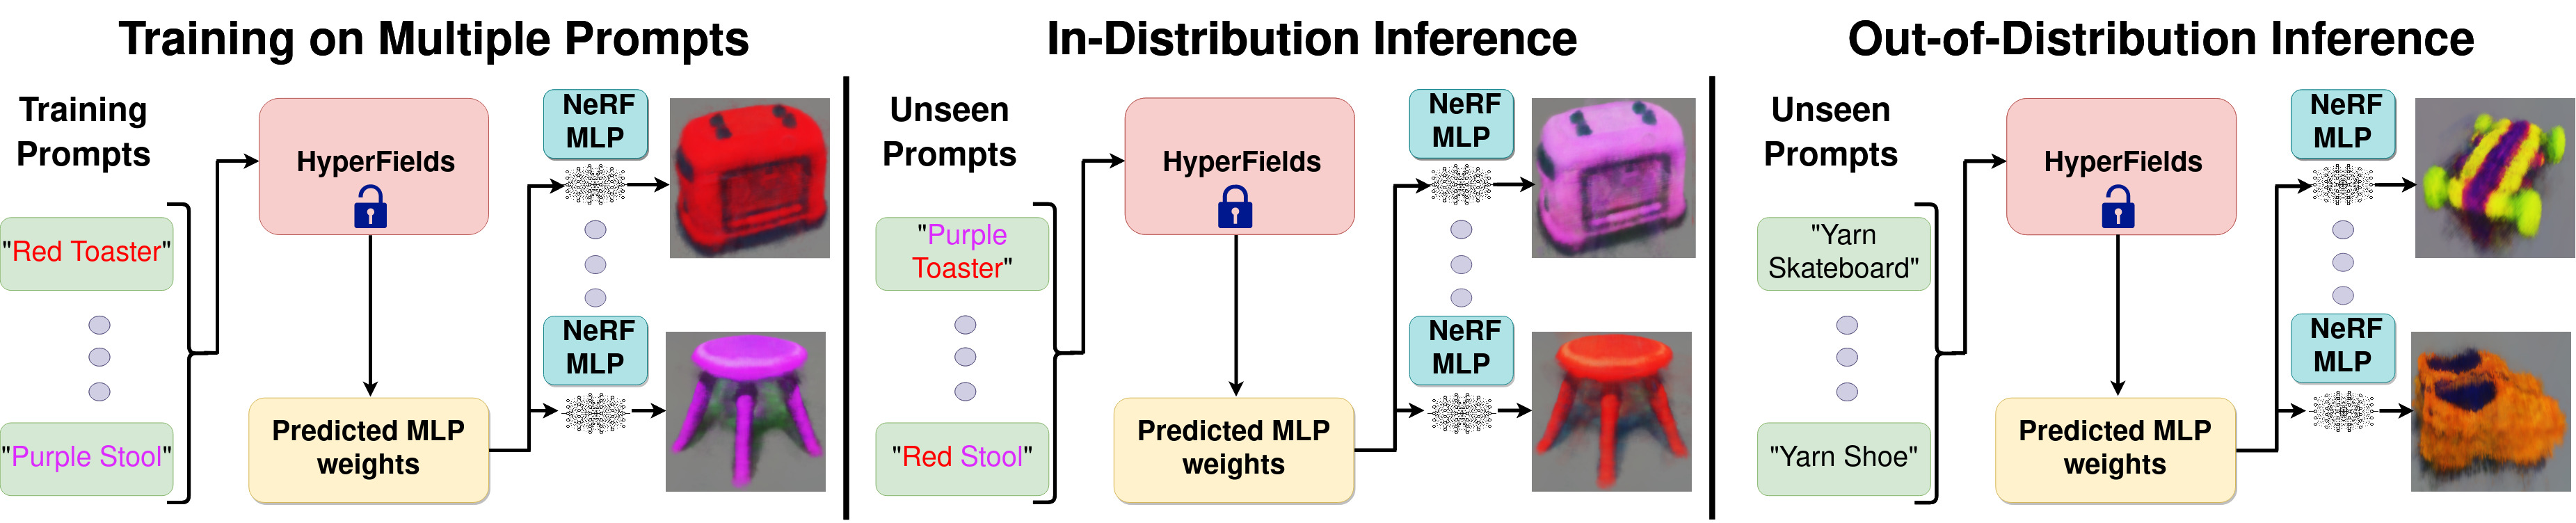}
% }]
\begin{figure*}
    \centering
    \includegraphics[width=18cm]{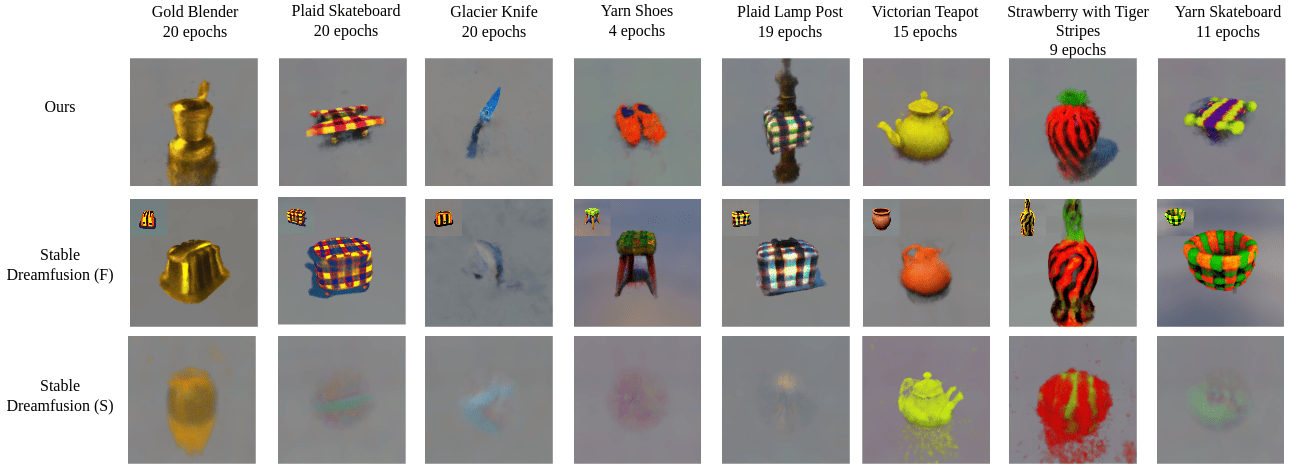}
    \caption{\textbf{Finetuning  to out of distribution geometry:} Our method accurately represents both the shape and texture using (at most) 20 epochs for all the objects, where the fine tuned (F) and trained from scratch (S) models are far from the desired prompt at the same number of epochs. Given a limited budget of 20 epochs, our method is faster while also being significantly better in terms of quality of the generated scene. The baseline trained from scratch (Stable Diffusion (S)) barely synthesizes any geometry in this amount of time and the finetune baseline does not alter the initialized geometry or completely erases it (as in ``Glacier Knife").}
    \label{fig:ood}
\end{figure*}

\section{Architecture Details}
\textbf{Baselines:} Our baseline is  6 layer MLP with skip connections every two layers. The hidden dimension is 64. We use an open-source \href{https://github.com/ashawkey/stable-dreamfusion}{re-implementation} \cite{stable-dreamfusion} of DreamFusion as both our baseline model and architecture predicted by the HyperNet, because the original DreamFusion works relies on Google's Imagen model which is not open-source. Unlike original DreamFusion, the re-implementation uses Stable Diffusion (instead of Imagen). We use Adam with a learning rate of 1e-4, with an epoch defined by 100 gradient descent steps.

\textbf{HyperFields:} The architecture is as described in Figure 2 in the main paper. The dynamic hypernetwork generates weights for a 6 layer MLP of hidden dimension 64. The transformer portion of the hypernetwork has 6 self-attention blocks, each with 12 heads with a head dimension of 16. We condition our model with BERT tokens, though we experiment with T5 and CLIP embeddings as well with similar but marginally worse success. Similar to the baseline we use Stable Diffusion for guidance, and optimize our model using Adam  with the a learning rate of 1e-4. We will release open-source code of our project in a future revision of the paper. 

\begin{figure*}
    \centering
    \includegraphics[width=1\textwidth]{images/compare_convergence_clear.png}
    \caption{\textbf{Comparing number of epochs to convergence:} On an average our method converges at least 5 times faster than both the fine tuned (F) and trained from scratch (S) baselines. As soon as a scene reasonably describes the given prompt we consider the model to have converged. In a few instances the baselines never generates a scene close to the text prompt, in which case we stop the run at 150 epochs.}
    \label{fig:oodconv}
\end{figure*}

\section{Convergence to Out of Distribution Geometry}
\label{sec:ood}
Figure 8 in the main paper shows a few examples (gold blender, plaid skateboard) of our model converging significantly faster than the baselines to a shape the model has not seen during training using the same optimization signal (Score Distillation Sampling). In this section we extend those results to more objects. \cref{fig:ood} shows that our model generates desirable shape and texture at very few epochs when compared to the fine-tuned baseline and the baseline trained from scratch. The fine tuned baselines are initialized to a NeRF that produces the same object predicted by our model zero shot. The initialization is illustrated in top left corner of the fine tuned baseline results, while similarly the zero shot results are on the top left corner of our model's results (Figure 3). 

In \cref{fig:oodconv} we compare the time to converge to a scene that reasonably represents the given prompt. From \cref{fig:oodconv}, we see that our model on an average converges 5 times faster than the baselines. From \cref{fig:oodvisual} we see that our model generates better quality scenes than the baselines. \textbf{Gold Blender:} the geometry for blender for both baselines is more similar to a cup, whereas ours has the shape of blender. \textbf{Plaid Skateboard:} The fine tuned model has the board mounted on box like shape, and the trained from scratch model is not as plaid-like, while our model generates a skateboard with a strong plaid texture to it. \textbf{Glacier Knife:} While the basic knife structure is present, the fine tuned model ignores the glacier texture. \textbf{Yarn Shoes:} All 3 models  model converge to reasonable shape and texture, although the shoes are kept mounted in the fine tuned model. \textbf{Plaid Lamp Post:} The trained from scratch model ignores the plaid attribute completely, and the synthesized lamppost is very small. The finetuned baseline simply creates a light from inside the toaster intialization. \textbf{Victorian Teapot:} The basic geometry seems to be present in all 3 models, however the handle is better placed in ours than in the baselines. \textbf{Strawberry with Tiger Stripes:} The shape of the fine tuned model looks more like a pineapple than a realistic strawberry, and the scratch baseline model does not have visible tiger stripes. \textbf{Yarn Skateboard:} With the yarn skateboard our geometry is more similar to a skateboard, while the fine tuned model does not move much beyond the bowl initialization, and the scratch baseline generates a plausible skateboard (albeit with some janused wheels) without any visible yarn texture.

\begin{figure*}
    \centering
    \includegraphics[width=18cm]{images/compare_converge_clear_big_fixed.png}
    \caption{\textbf{Comparing geometries at convergence:} In this experiment we simply let the baselines (row 2 and 3) in Figure \cref{fig:ood} continue training till the scene generated is reasonably similar to the text prompt. However, despite training the baseline models longer, in quite a few cases the geometry/texture generated by our method is better than the baselines. We compare and discuss our quality advantage in \cref{sec:ood}. The inset figures top left hand side are the zero shot predictions by our model, and in the case of the fine tunes baseline it is the scene the NeRF is initially trained on.}
    \label{fig:oodvisual}
\end{figure*}

\section{Packing}
In \cref{fig:simplepack} and \cref{fig:complexpack} we show various scenes we were able to train/pack simultaneously into a single hypernetwork, over a set of simple color prompts, as well as a diverse and varying set of complex prompts. 

\begin{figure*}
    \centering
    \includegraphics[width=\textwidth]{images/simplepack.png}
    \caption{\textbf{Simple Prompt Packing.} We show the HyperFields ability to pack 10 different objects across 8 different colors.}
    \label{fig:simplepack}
\end{figure*}

\begin{figure*}
    \centering
    \includegraphics[width=\textwidth]{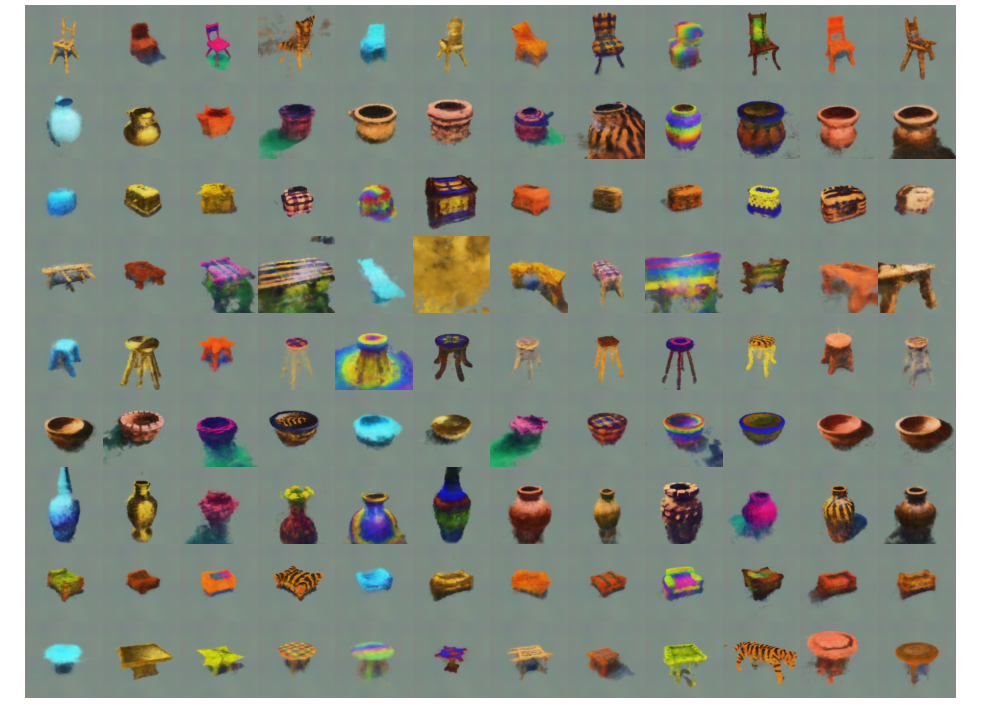}
    \caption{\textbf{Complex Prompt Packing.} Our dynamic hypernetwork is able to pack 9 different objects across 12 different prompts for a total of 108 scenes. Dynamic hypetnetwork coupled with NeRF distillation enables packing these scenes into one network.}
    \label{fig:complexpack}
\end{figure*}

\subsection{Interpolation}
\label{sec:interpolation}

\begin{figure*}
    \centering
    \includegraphics[width=\textwidth]{images/interpolation.png}
    \caption{\ourmethod{} learns a smooth mapping of the BERT latent space, which allows us to interpolate between scenes through interpolating the hypernet-predicted conditioning token or the predicted NeRF weights.}
    % We show that interpolating along different NeRF layer depths e.g. layers 1-2 (L1-L2) corresponds to interpolating different levels of semantic abstraction.}
    \label{fig:interpolation}
\end{figure*}

Fig.~\ref{fig:interpolation} demonstrates that we can interpolate the hypernetwork predictions in a variety of ways to achieve a smooth mapping between different packed NeRF scenes. Interpolating either the hypernet-predicted conditioning tokens (``Hypernet Conditioning") or the hypernet-predicted NeRF parameters (``NeRF Parameters (All)") generate smooth interpolations of the scenes. Note that the orange colour interpolates to purple through a natural spectrum (red, pink). These results prove that \ourmethod{} learns a smooth function of the input BERT tokens, and more importantly, learns a function which preserves the semantic meaning of the input text. 

\section{User Study}
\label{sec:study}

\section{BERT Token Interpolation}

\begin{figure*}
    \centering
    \includegraphics[width=\textwidth]{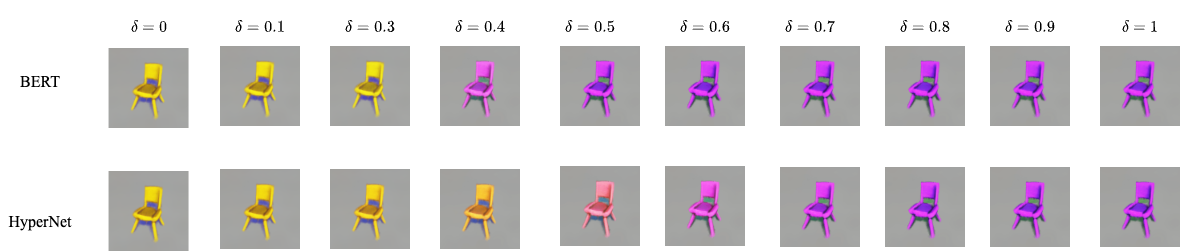}
    \caption{\textbf{BERT Token Interpolation.} We show results of interpolating the BERT tokens corresponding to the prompts ``yellow chair" and ``purple chair". In contrast, interpolation on the level of the hypernetwork (``HyperNet") is more smoother than interpolating the BERT tokens. }
    \label{fig:bertinterpolation}
\end{figure*}

Another option for interpolation is to interpolate the input BERT embeddings fed in the our Dynamic HyperNet. We show results in \cref{fig:bertinterpolation} where we interpolate across two chair colors in a Dynamic HyperNet trained on only chair colors. The interpolation is highly non-smooth, with a single intermediate color shown at $\delta=0.4$ and discontinuities on either end at $\delta-0.3$ and $\delta=0.5$. On the other hand, our HyperNet token interpolation shown in Figure 10 demonstrates a smooth and gradual transition of colors across the interpolation range. This demonstrates that our HyperNet learns a smoother latent space of NeRFs than the original BERT tokens correspond to.

\Section{Additional Quantitative Evaluation}
Furthermore, we report CLIP precision and recall scores (retrieving the 3 nearest-neighbors), along with KID, SSIM scores. We compare with the Stable DreamFusion baselines trained for the same computational budget for the out-of-distribution scenes from  shown in Fig. \ref{fig:ood}.

{\small
\bibliographystyle{ieee_fullname}
\bibliography{supp_bib}
}
\end{document}
